# Supplementary material for: Cayley graphs of order 16p are hamiltonian
Source: arXiv:1104.0081 ancillary file (2011-04-04)
Supplement: Supplementary file 1 [file 48.pdf]

# CAYLEY GRAPHS OF ORDER 48 ARE HAMILTONIAN

STEPHEN J. CURRAN, DAVE WITTE MORRIS, AND JOY MORRIS

Abstract. We prove that if $|G| = 48$, and the Sylow 3-subgroups of $G$ are not normal, then every connected Cayley graph on $G$ has a hamiltonian cycle.

## A1. Introduction

This (unpublished) appendix to [14] provides a proof of Proposition 3.4 of that paper:

**Proposition 3.4.** *If $|G| = 48$, and the Sylow 3-subgroups of $G$ are not normal, then every connected Cayley graph on $G$ has a hamiltonian cycle.*

## Contents

A1. Introduction 1
A2. Preliminaries on hamiltonian cycles in Cayley graphs 1
A3. Cayley graphs on the group $S_4 \times \mathbb{Z}_2$ 2
A4. Groups of order 48 and their generating sets 7
A5. Proof of Proposition 3.4 10
Additional references 15

*Acknowledgments.* This research was partially supported by a grant from the Natural Sciences and Engineering Research Council of Canada. Most of the work was carried out during a visit of S. J. C. to the University of Lethbridge.

## A2. Preliminaries on hamiltonian cycles in Cayley graphs

(A2.1) **Lemma** (Jungreis-Friedman [16, Lem. 7.1], [10, Lem. 2.18]). *Let $S$ be a minimal generating set for the group $G$. If there exist two distinct generators $s_1, s_2 \in S$ such that:*

- $|s_1 s_2| = |G|/|\langle S - \{s_1\}\rangle|$,
- $\langle s_1 s_2 \rangle \cap \langle S - \{s_1\}\rangle = \{e\}$, *and*
- *there is a hamiltonian cycle in* $\mathrm{Cay}\big(\langle S - \{s_1\}\rangle; S - \{s_1\}\big)$,

*then there is a hamiltonian cycle in* $\mathrm{Cay}(G; S)$.

(A2.2) **Lemma** (cf. [12, Lem. 5.1]). *Suppose*

- *$H$ is a cyclic subgroup of $G$,*
- *$(s_1, s_2, \ldots, s_n)$ is a hamiltonian cycle in the quotient $H\backslash \mathrm{Cay}(G; S)$, and*
- *the product $s_1 s_2 \cdots s_n$ generates $H$.*

*Then $(s_1, s_2, \ldots, s_n)^{|H|}$ is a hamiltonian cycle in* $\mathrm{Cay}(G; S)$.

*Date*: April 4, 2011.

(A2.3) *Notation.* We use $\overrightarrow{\mathrm{Cay}}(G;S)$ to denote the *Cayley digraph* of $G$ with respect to the generating set $S$. Note that this is a *digraph*, not an undirected graph.

Here is a very old result that deserves to be better known:

(A2.4) **Theorem** (R. A. Rankin [17, Thm. 3.1(i)]). *If* $\langle a,b\rangle = G$ *and* $(ab^{-1})^2 = e$, *then* $\overrightarrow{\mathrm{Cay}}\big(G;\{a,b\}\big)$ *has a directed hamiltonian cycle.*

(A2.5) **Corollary.** *Suppose there exist* $t,a,b \in S \cup S^{-1}$, *such that*

- $\langle t,a,b\rangle = G$,
- $|ab^{-1}| = 2$, *and*
- $|G/\langle at,bt\rangle| = 2$.

*Then* $\mathrm{Cay}(G;S)$ *has a hamiltonian cycle.*

**Proof.** Let $H = \langle at,bt\rangle$. Then, since $(at)(bt)^{-1} = ab^{-1}$ has order 2, Theorem A2.4 tells us that the Cayley digraph $\overrightarrow{\mathrm{Cay}}\big(H;\{at,bt\}\big)$ has a directed hamiltonian cycle; this hamiltonian cycle is of the form

$$(s_1t, s_2t, \ldots, s_nt), \text{ where } s_i \in \{a,b\} \subset S \cup S^{-1}, \text{ so } s_i \in S \cup S^{-1}.$$

Furthermore, since, by assumption, $H$ has index 2 in $G$, we see that $H$ and $Ht$ are the only cosets of $H$. Thus, it is clear that $(s_1,t,s_2,\ldots,s_n,t)$ is a hamiltonian cycle in $\mathrm{Cay}(G;S)$. (This is a case of the "skewed generators argument" [12, Lem. 5.1].) □

## A3. Cayley graphs on the group $S_4 \times \mathbb{Z}_2$

(A3.1) **Proposition.** *If* $G \cong S_4 \times \mathbb{Z}_2$, *then every Cayley graph on* $G$ *has a hamiltonian cycle.*

**Proof.** For convenience, we represent $G$ as the subgroup $S_4 \times \langle (5,6)\rangle$ of $S_6$.

Unfortunately, $G$ has 53 different minimal generating sets, up to automorphisms of $G$. (These were found by computer search.) Each of these generating sets will be treated individually.

There are only 4 2-element generating sets:

(2.1) $S = \{(3,4),(1,2,3)(5,6)\}$

Letting $a = (3,4)$ and $b = (1,2,3)(5,6)$, a hamiltonian cycle in $\mathrm{Cay}(G;S)$ is:

$$\big((b^5,a)^2,(b^{-5},a)^2\big)^2.$$

This passes through the vertices of $\mathrm{Cay}(G;S)$ in the order:

$(1), (1,2,3)(5,6), (1,3,2), (5,6), (1,2,3), (1,3,2)(5,6), (1,4,3,2)(5,6), (1,4),$
$(1,4,2,3)(5,6), (1,4,3,2), (1,4)(5,6), (1,4,2,3), (1,3)(2,4), (1,2,4)(5,6),$
$(2,4,3), (1,3)(2,4)(5,6), (1,2,4), (2,4,3)(5,6), (2,3)(5,6), (1,3), (1,2)(5,6),$
$(2,3), (1,3)(5,6), (1,2), (1,2)(3,4), (1,3,4)(5,6), (2,4,3), (1,2)(3,4)(5,6),$
$(1,3,4), (2,3,4)(5,6), (2,4)(5,6), (1,2,4,3), (1,3,2,4)(5,6), (2,4), (1,2,4,3)(5,6),$
$(1,3,2,4), (1,4)(2,3), (1,4,3)(5,6), (1,4,2), (1,4)(2,3)(5,6), (1,4,3), (1,4,2)(5,6),$
$(1,3,4,2)(5,6), (1,2,3,4), (3,4)(5,6), (1,3,4,2), (1,2,3,4)(5,6), (3,4), (1).$

(2.2) $S = \{(3,4),(1,2,3,4)(5,6)\}$
Letting $a = (3,4)$ and $b = (1,2,3,4)(5,6)$, a hamiltonian cycle in $\mathrm{Cay}(G/\mathbb{Z}_2;S)$ is:

$$\big((a,b)^2, a, b^{-1}, (a,b^3,a,b)^3\#, b^{-1}\big).$$

This passes through the elements of $G/\mathbb{Z}_2 \cong S_4$ in the order:

$(1),(3,4),(1,2,3),(1,2,4,3),(1,3,2),(1,4,3,2),(1,3)(2,4),(1,4,2,3),(2,4,3),$
$(1,2),(1,3,4),(1,4),(2,3,4),(2,4),(1,2)(3,4),(1,3),(1,4)(2,3),$
$(1,3,2,4),(1,4,2),(1,3,4,2),(1,4,3),(2,3),(1,2,4),(1,2,3,4),(1).$

Since there are an odd number of $b$ and $b^{-1}$-edges (combined), it is clear that the endpoint in $G$ is $(5,6)$, so the Factor Group Lemma (2.1) provides a hamiltonian cycle in $\mathrm{Cay}(G;S)$.

(2.3) $S = \{(2,3,4)(5,6),(1,2,3,4)\}$
Theorem A2.4 applies with $a = (2,3,4)(5,6)$ and $b = (1,2,3,4)$ (so $ab^{-1} = (1,4)$ has order 2).

(2.4) $S = \{(1,2,3,4),(1,2,4,3)(5,6)\}$
Letting $a = (1,2,3,4)$ and $b = (1,2,4,3)(5,6)$, a hamiltonian cycle in $\mathrm{Cay}(G/\mathbb{Z}_2;S)$ is:

$$\big(b^3, a^{-3}, b^{-1}, a^3, b^{-1}, a^{-2}, b, a^{-1}, b^{-1}, a^2, b^{-1}, a, b^{-1}, a^3\big).$$

This passes through the elements of $G/\mathbb{Z}_2 \cong S_4$ in the order:

$(1),(1,2,4,3),(1,4)(2,3),(1,3,4,2),(1,2,4),(2,3),(1,4,3),(1,2),(1,3,4),$
$(1,4,2,3),(2,4,3),(1,3),(1,2)(3,4),(2,4),(1,2,3),(3,4),(1,3,2),$
$(1,4),(2,3,4),(1,3,2,4),(1,4,2),(1,2,3,4),(1,3)(2,4),(1,4,3,2),(1).$

Since there are an odd number of $b$ and $b^{-1}$-edges (combined), it is clear that the endpoint of this cycle in $G$ is $(5,6)$, so the Factor Group Lemma (2.1) provides a hamiltonian cycle in $\mathrm{Cay}(G;S)$.

There are 10 4-element generating sets, but all of them contain either an element of $\mathbb{Z}_2$ (so Lemma 2.6(1) applies), or two generators whose product is in $\mathbb{Z}_2$, so Corollary 2.2 applies.

There are 39 3-element generating sets (of which all but 12 can be handled very easily):

(3.1) $S = \{(5,6),(3,4),(1,2,3)\}$
$(5,6) \in \mathbb{Z}_2$, so Lemma 2.6(1) applies.

(3.2) $S = \{(5,6),(3,4),(1,2,3,4)\}$
$(5,6) \in \mathbb{Z}_2$, so Lemma 2.6(1) applies.

(3.3) $S = \{(5,6),(2,3,4),(1,2,3,4)\}$
$(5,6) \in \mathbb{Z}_2$, so Lemma 2.6(1) applies.

(3.4) $S = \{(5,6),(1,2,3,4),(1,2,4,3)\}$
$(5,6) \in \mathbb{Z}_2$, so Lemma 2.6(1) applies.

(3.5) $S = \{(3,4),(3,4)(5,6),(1,2,3)\}$
Apply Corollary 2.2 with $s = (3,4)$, $t = (3,4)(5,6)$, and $N = \mathbb{Z}_2$.

(3.6) $S = \{(3,4),(2,3),(1,2)(5,6)\}$
Apply Corollary A2.5 with $t = (2,3)$, $a = (1,2)(5,6)$, and $b = (3,4)$.

(3.7) $S = \{(3,4),(2,3),(1,2)(3,4)(5,6)\}$
Apply Corollary A2.5 with $t = (2,3)$, $a = (1,2)(3,4)(5,6)$, and $b = (3,4)$.

(3.8) $S = \{(3,4),(2,3),(1,3)(5,6)\}$
Letting $a = (3,4)$, $b = (2,3)$, and $c = (1,3)(5,6)$, a hamiltonian cycle in $\mathrm{Cay}(G;S)$ is:

$$\Big(\big((b,a)^3\#,c\big)^2, \big((a,b)^3\#,c\big)^2\Big)^2.$$

This passes through the vertices in the order:

$(1), (2,3), (2,4,3), (2,4), (2,3,4), (3,4), (1,3,4)(5,6), (1,2,3,4)(5,6), (1,2,4)(5,6),$
$(1,3,2,4)(5,6), (1,4)(2,3)(5,6), (1,4)(5,6), (1,4,3), (1,3), (1,2,3), (1,2,4,3), (1,3)(2,4),$
$(1,4,2,3), (1,4,2)(5,6), (1,3,4,2)(5,6), (1,2)(3,4)(5,6), (1,2)(5,6), (1,3,2)(5,6),$
$(1,4,3,2)(5,6), (1,4)(2,3), (1,4), (1,3,4), (1,2,3,4), (1,2,4), (1,3,2,4), (2,4,3)(5,6),$
$(2,4)(5,6), (2,3,4)(5,6), (3,4)(5,6), (5,6), (2,3)(5,6), (1,3,2), (1,4,3,2), (1,4,2),$
$(1,3,4,2), (1,2)(3,4), (1,2), (1,2,3)(5,6), (1,2,4,3)(5,6), (1,3)(2,4)(5,6), (1,4,2,3)(5,6),$
$(1,4,3)(5,6), (1,3)(5,6), (1).$

(3.9) $S = \{(3,4),(2,3),(1,3)(2,4)(5,6)\}$
Letting $a = (3,4)$, $b = (2,3)$, and $c = (1,3)(2,4)(5,6)$, a hamiltonian cycle in $\mathrm{Cay}(G;S)$ is:

$$\big((b,a)^3\#,c,((a,b)^3\#,c)^2,(b,a)^3\#,c\big)^2.$$

This passes through the vertices in the order:

$(1), (2,3), (2,4,3), (2,4), (2,3,4), (3,4), (1,3,2,4)(5,6), (1,4)(2,3)(5,6), (1,4)(5,6),$
$(1,3,4)(5,6), (1,2,3,4)(5,6), (1,2,4)(5,6), (1,4,3), (1,3), (1,2,3), (1,2,4,3), (1,3)(2,4),$
$(1,4,2,3), (1,2)(5,6), (1,3,2)(5,6), (1,4,3,2)(5,6), (1,4,2)(5,6), (1,3,4,2)(5,6),$
$(1,2)(3,4)(5,6), (1,4)(2,3), (1,4), (1,3,4), (1,2,3,4), (1,2,4), (1,3,2,4), (3,4)(5,6), (5,6),$
$(2,3)(5,6), (2,4,3)(5,6), (2,4)(5,6), (2,3,4)(5,6), (1,3,2), (1,4,3,2), (1,4,2), (1,3,4,2),$
$(1,2)(3,4), (1,2), (1,4,2,3)(5,6), (1,4,3)(5,6), (1,3)(5,6), (1,2,3)(5,6), (1,2,4,3)(5,6),$
$(1,3)(2,4)(5,6), (1).$

(3.10) $S = \{(3,4),(2,3)(5,6),(1,2)\}$
Apply Corollary A2.5 with $t = (2,3)(5,6)$, $a = (1,2)$, and $b = (3,4)$.

(3.11) $S = \{(3,4),(2,3)(5,6),(1,2)(3,4)\}$
Apply Lemma A2.1with $s_1 = (3,4)$ and $s_2 = (2,3)(5,6)$ (so $|s_1 s_2| = 6$).

(3.12) $S = \{(3,4),(2,3)(5,6),(1,2)(3,4)(5,6)\}$
Apply Lemma A2.1 with $s_1 = (3,4)$ and $s_2 = (2,3)(5,6)$ (so $|s_1 s_2| = 6$).

(3.13) $S = \{(3,4),(2,3)(5,6),(1,2,3)\}$
Letting $a = (3,4)$, $b = (2,3)(5,6)$, and $c = (1,2,3)$, a hamiltonian cycle in $\mathrm{Cay}(G/\mathbb{Z}_2;S)$ is:

$$\big(b,c^{-2},a,(c^2,a)^2,c^{-2},a,c^2,a,(c^{-2},a)^2,c^{-2}\big).$$

This passes through the elements of $G/\mathbb{Z}_2 \cong S_4$ in the order:

$$(1), (2,3), (1,3), (1,2), (1,2)(3,4), (1,3,4), (2,3,4), (2,4), (1,2,4,3),$$
$$(1,3,2,4), (1,4)(2,3), (1,4,3), (1,4,2), (1,3,4,2), (3,4), (1,2,3,4), (1,2,4),$$
$$(2,4,3), (1,3)(2,4), (1,4,2,3), (1,4), (1,4,3,2), (1,3,2), (1,2,3), (1).$$

Since there are an odd number of $b$-edges, it is clear that the endpoint in $G$ is $(5,6)$, so the Factor Group Lemma (2.1) applies.

(3.14) $S = \{(3,4), (2,3)(5,6), (1,2,4,3)\}$
Apply Lemma A2.1 with $s_1 = (3,4)$ and $s_2 = (2,3)(5,6)$ (so $|s_1 s_2| = 6$).

(3.15) $S = \{(3,4), (2,3)(5,6), (1,2,4)\}$
Letting $a = (3,4)$, $b = (2,3)(5,6)$, and $c = (1,2,4)$, a hamiltonian cycle in $\mathrm{Cay}(G/\mathbb{Z}_2)$ is:

$$\big(b, c^2, a, c^{-2}, a, (c^2, a)^2, (c^{-2}, a)^2, c^2, a, c^{-2}\big).$$

This passes through the elements of $G/\mathbb{Z}_2 \cong S_4$ in the order:

$$(1), (2,3), (1,2,3,4), (1,4,2,3), (1,3)(2,4), (1,3,4), (1,3,2), (1,4,3,2), (3,4),$$
$$(1,2,4,3), (1,2,3), (1,4)(2,3), (2,3,4), (2,4), (1,4), (1,2), (1,2)(3,4),$$
$$(2,4,3), (1,4,3), (1,3), (1,3,2,4), (1,3,4,2), (1,4,2), (1,2,4), (1).$$

Since there are an odd number of $b$-edges, it is clear that the endpoint in $G$ is $(5,6)$, so the Factor Group Lemma (2.1) applies.

(3.16) $S = \{(3,4), (2,3)(5,6), (1,3)(2,4)\}$
Apply Lemma A2.1 with $s_1 = (3,4)$ and $s_2 = (2,3)(5,6)$ (so $|s_1 s_2| = 6$).

(3.17) $S = \{(3,4), (2,3)(5,6), (1,3)(2,4)(5,6)\}$
Apply Lemma A2.1 with $s_1 = (3,4)$ and $s_2 = (2,3)(5,6)$ (so $|s_1 s_2| = 6$).

(3.18) $S = \{(3,4), (2,3,4), (1,2)(5,6)\}$
Apply Lemma A2.1 with $s_1 = (3,4)$ and $s_2 = (2,3,4)$ (so $|s_1 s_2| = 2$).

(3.19) $S = \{(3,4), (2,3,4), (1,2)(3,4)(5,6)\}$
Apply Lemma A2.1 with $s_1 = (3,4)$ and $s_2 = (2,3,4)$ (so $|s_1 s_2| = 2$).

(3.20) $S = \{(3,4), (2,3,4), (1,3,4)(5,6)\}$
Apply Lemma A2.1 with $s_1 = (3,4)$ and $s_2 = (2,3,4)$ (so $|s_1 s_2| = 2$).

(3.21) $S = \{(3,4), (2,3,4), (1,3)(2,4)(5,6)\}$
Apply Lemma A2.1 with $s_1 = (3,4)$ and $s_2 = (2,3,4)$ (so $|s_1 s_2| = 2$).

(3.22) $S = \{(3,4), (2,3,4), (1,3,2,4)(5,6)\}$
Apply Lemma A2.1 with $s_1 = (3,4)$ and $s_2 = (2,3,4)$ (so $|s_1 s_2| = 2$).

(3.23) $S = \{(3,4), (2,3,4)(5,6), (1,2)(3,4)\}$
Apply Lemma A2.1 with $s_1 = (3,4)$ and $s_2 = (2,3,4)(5,6)$ (so $|s_1 s_2| = 2$).

(3.24) $S = \{(3,4), (2,3,4)(5,6), (1,2)(3,4)(5,6)\}$
Apply Lemma A2.1 with $s_1 = (3,4)$ and $s_2 = (2,3,4)(5,6)$ (so $|s_1 s_2| = 2$).

(3.25) $S = \{(3,4), (2,3,4)(5,6), (1,2,3)\}$
Apply Lemma A2.1 with $s_1 = (3,4)$ and $s_2 = (2,3,4)(5,6)$ (so $|s_1 s_2| = 2$).

(3.26) $S = \{(3,4), (2,3,4)(5,6), (1,3,4)(5,6)\}$
Apply Lemma A2.1 with $s_1 = (3,4)$ and $s_2 = (2,3,4)(5,6)$ (so $|s_1 s_2| = 2$).

(3.27) $S = \{(3,4), (2,3,4)(5,6), (1,3)(2,4)\}$
Apply Lemma A2.1 with $s_1 = (3,4)$ and $s_2 = (2,3,4)(5,6)$ (so $|s_1 s_2| = 2$).

(3.28) $S = \{(3,4), (2,3,4)(5,6), (1,3)(2,4)(5,6)\}$
Apply Lemma A2.1 with $s_1 = (3,4)$ and $s_2 = (2,3,4)(5,6)$ (so $|s_1 s_2| = 2$).

(3.29) $S = \{(3,4), (1,2)(3,4)(5,6), (1,2,3)\}$
Apply Lemma A2.1 with $s_1 = (3,4)$ and $s_2 = (1,2)(3,4)(5,6)$ (so $|s_1 s_2| = 2$).

(3.30) $S = \{(3,4), (1,2)(3,4)(5,6), (1,2,3,4)\}$ Letting $a = (3,4)$, $b = (1,2)(3,4)(5,6)$, and $c = (1,2,3,4)$, a hamiltonian cycle in $\mathrm{Cay}(G; S)$ is:

$$\big(b, (a, c^{-1}, (a,c)^2)^2\#, b, (a, c^{-1}, a, c, a, c^{-1})^2\#\big)^2.$$

This passes through the vertices of the graph in the order:

(1), (1,2)(3,4)(5,6), (1,2)(5,6), (2,4,3)(5,6), (2,3)(5,6), (1,2,4)(5,6), (2,3,4)(5,6), (1,3)(2,4)(5,6), (1,4,2,3)(5,6), (1,3,4)(5,6), (1,4)(5,6), (2,3,4)(5,6), (2,4)(5,6), (2,3,4), (1,2,4), (2,3), (2,4,3), (1,2), (1,2)(3,4), (2,4), (2,3,4), (1,4), (1,3,4), (1,4,2,3), (1,3)(2,4), (1,4)(2,3)(5,6), (1,3,2,4)(5,6), (1,2,3)(5,6), (1,2,4,3)(5,6), (1,3,2)(5,6), (1,4,3,2)(5,6), (5,6), (3,4)(5,6), (1,4,2)(5,6), (1,3,4,2)(5,6), (1,4,3)(5,6), (1,3)(5,6), (1,4,3,2), (1,3,2), (1,2,4,3), (1,2,3), (1,3,2,4), (1,4)(2,3), (1,3), (1,4,3), (1,3,4,2), (1,4,2), (3,4), (1).

(3.31) $S = \{(3,4), (1,2,3), (1,3)(2,4)(5,6)\}$
Letting $a = (3,4)$, $b = (1,2,3)$, and $c = (1,3)(2,4)(5,6)$, a hamiltonian cycle in $\mathrm{Cay}(G/\mathbb{Z}_2 : S)$ is:

$$\big((a, b^2)^2, c, (a, b^2)^3, a, b, a, b^{-2}, a, b^2\big).$$

This passes through the elements of $G/\mathbb{Z}_2 \cong S_4$ in the order:

(1), (3,4), (1,2,3,4), (1,3,4,2), (1,4,2), (1,4,3), (1,4)(2,3), (1,2)(3,4), (1,2), (1,3), (2,3), (2,4,3), (1,2,4), (1,3)(2,4), (1,4,2,3), (1,4,3,2), (1,4), (1,3,4), (2,3,4), (2,4), (1,3,2,4), (1,2,4,3), (1,2,3), (1,3,2),(1).

Since there are an odd number of $c$-edges, it is clear that the endpoint in $G$ is $(5,6)$, so the Factor Group Lemma (2.1) applies.

(3.32) $S = \{(3,4), (1,2,3), (1,3,2,4)(5,6)\}$
Apply Lemma A2.1 with $s_1 = (3,4)$ and $s_2 = (1,3,2,4)(5,6)$ (so $|s_1 s_2| = 2$).

(3.33) $S = \{(3,4), (1,2,3,4), (1,3)(2,4)(5,6)\}$
Letting $a = (3,4)$, $b = (1,2,3,4)$, and $c = (1,3)(2,4)(5,6)$, a hamiltonian cycle in $\mathrm{Cay}(G; S)$ is:

$$\big(c, (b, a, (b^{-1}, a)^2)^2\#, c, ((b,a)^2, b^{-1}, a)^2\#\big)^2.$$

This passes through the vertices in the order:

$(1), (1,3)(2,4)(5,6), (1,4,3,2)(5,6), (1,3,2)(5,6), (1,2,4,3)(5,6), (1,2,3)(5,6), (3,4)(5,6), (5,6), (1,2,3,4)(5,6), (1,2,4)(5,6), (2,3)(5,6), (2,4,3)(5,6), (1,4,2,3)(5,6), (1,2), (1,3,4), (1,4), (2,3,4), (2,4), (1,4)(2,3), (1,3,2,4), (1,4,2), (1,3,4,2), (1,4,3), (1,3), (1,2)(3,4), (1,4)(2,3)(5,6), (2,4)(5,6), (2,3,4)(5,6), (1,4)(5,6), (1,3,4)(5,6), (1,2)(5,6), (1,2)(3,4)(5,6), (1,3)(5,6), (1,4,3)(5,6), (1,3,4,2)(5,6), (1,4,2)(5,6), (1,3,2,4)(5,6), (3,4), (1,2,3), (1,2,4,3), (1,3,2), (1,4,3,2), (1,3)(2,4), (1,4,2,3), (2,4,3), (2,3), (1,2,4), (1,2,3,4), (1)$.

(3.34) $S = \{(3,4), (1,2,3,4), (1,4)(2,3)(5,6)\}$
Apply Corollary A2.5 with $t = (3,4)$, $a = (1,2,3,4)^{-1} = (1,4,3,2)$, and $b = (1,4)(2,3)(5,6)$.

(3.35) $S = \{(2,3,4), (1,2)(3,4)(5,6), (1,2,3,4)\}$
Apply Lemma A2.1 with $s_1 = (2,3,4)$ and $s_2 = (1,2)(3,4)(5,6)$ (so $|s_1 s_2| = 6$).

(3.36) $S = \{(2,3,4), (1,2)(3,4)(5,6), (1,3,2,4)\}$
Letting $a = (2,3,4)$, $b = (1,2)(3,4)(5,6)$, and $c = (1,3,2,4)$, a hamiltonian cycle in $\mathrm{Cay}(G/\mathbb{Z}_2; S)$ is:

$$\big(c^{-1}, a, c^3, a, c, b, a^{-1}, c^{-3}, a, c, b, c^{-1}, a^2, c^3, a, c, b\big).$$

This passes through the elements of $G/\mathbb{Z}_2 \cong S_4$ in the order:

$$(1), (1,4,2,3), (1,2,4,3), (1,4,2), (2,3), (1,3,4), (1,4)(2,3), (3,4), (1,2), (1,4,3,2), (1,2,4), (1,3), (2,3,4), (2,4,3), (1,3,4,2), (1,4), (1,2,3), (1,3)(2,4), (1,4,3), (2,4), (1,3,2), (1,2,3,4), (1,3,2,4), (1,2)(3,4), (1).$$

Since there are an odd number of $b$-edges, it is clear that the endpoint in $G$ is $(5,6)$, so the Factor Group Lemma (2.1) applies.

(3.37) $S = \{(2,3,4), (1,2,3,4), (1,2,3,4)(5,6)\}$
Apply Corollary 2.2 with $s = (1,2,3,4)$, $t = (1,2,3,4)(5,6)$, and $N = \langle (5,6) \rangle$.

(3.38) $S = \{(1,2)(3,4)(5,6), (1,2,3,4), (1,2,4,3)\}$
Apply Lemma A2.1 with $s_1 = (1,2)(3,4)(5,6)$ and $s_2 = (1,2,3,4)$ (so $|s_1 s_2| = 2$).

(3.39) $S = \{(1,2)(3,4)(5,6), (1,2,3,4), (1,3,2,4)\}$
Apply Lemma A2.1 with $s_1 = (1,2)(3,4)(5,6)$ and $s_2 = (1,2,3,4)$ (so $|s_1 s_2| = 2$). □

## A4. Groups of order 48 and their generating sets

(A4.1) **Lemma.** *There are exactly* 10 *groups of order* 48 *that have no normal Sylow* 3*-subgroup:*

(1) 6 *groups in which the Sylow* 2*-subgroup is normal:*
  (a) $\mathbb{Z}_3 \ltimes (\mathbb{Z}_4)^2 = \langle x \rangle \ltimes \langle y, z \rangle$ *with* $y^x = z$ *and* $z^x = y^{-1} z^{-1}$,
  (b) $A_4 \times \mathbb{Z}_4 \cong \big(\mathbb{Z}_3 \ltimes (\mathbb{Z}_2)^2\big) \times \mathbb{Z}_4 = \big(\langle x \rangle \ltimes \langle y, y' \rangle\big) \times \langle w \rangle$, *where* $y^x = y'$ *and* $(y')^x = yy'$,
  (c) $A_4 \times (\mathbb{Z}_2)^2 = \big(\mathbb{Z}_3 \ltimes (\mathbb{Z}_2)^2\big) \times (\mathbb{Z}_2)^2 = \big(\langle x \rangle \ltimes \langle y, y' \rangle\big) \times \langle z, z' \rangle$,
  (d) $\mathbb{Z}_3 \ltimes \big((\mathbb{Z}_2)^2\big)^2 = \langle x \rangle \ltimes \big(\langle y, y' \rangle \times \langle z, z' \rangle\big)$, *where* $\mathbb{Z}_3$ *acts nontrivially on each* $(\mathbb{Z}_2)^2$,
  (e) $\mathrm{SL}_2(3) \times \mathbb{Z}_2 \cong (\mathbb{Z}_3 \ltimes Q_8) \times \mathbb{Z}_2 = \big(\langle x \rangle \ltimes \langle i, j \rangle\big) \times \langle w \rangle$,

(f) $\dfrac{(\mathbb{Z}_3 \ltimes Q_8) \times \mathbb{Z}_4}{\langle (e, i^2, w^2) \rangle} \cong \mathbb{Z}_2 \ltimes \mathrm{SL}_2(3)$, *where* $\mathbb{Z}_2$ *acts on* $\mathrm{SL}_2(3)$ *via an inner automorphism.*

(2) 4 *groups in which the Sylow* 2*-subgroups are not normal:*

(a) $S_4 \times \mathbb{Z}_2$,

(b) $\mathbb{Z}_4 \ltimes A_4$, *where* $\mathbb{Z}_4$ *acts via conjugation by an odd permutation in* $S_4$,

(c) $\mathrm{GL}_2(3) \cong D_6 \ltimes Q_8$, *where* $i^f = -j$, $j^f = -i$, $k^f = -k$, $i^t = j$, $j^t = k$, $k^t = i$,

(d) $\widetilde{S}_4 = \dfrac{\mathbb{Z}_4 \ltimes (\mathbb{Z}_3 \ltimes Q_8)}{\langle (x^2, e, i^2) \rangle}$, *where* $x$ *inverts* $\mathbb{Z}_3 = \langle y \rangle$ *and acts on* $Q_8$ *like* $f$ *in the preceding group.*

**Comments on the proof.** The computer program GAP [15] can quickly find all 10 of the above groups (because it has a built-in list of the 52 groups of order 48).

Alternatively, the proof is not a difficult exercise. For (1), one looks through the list of 14 groups of order 16, to find the ones that have an automorphism of order 3. In (2), it is helpful to know that there must be a normal subgroup of order 8 (because it is a standard exercise to prove that every group of order 48 has a normal subgroup of order 8 or 16); this subgroup must have an automorphism of order 3, so it is either $Q_8$ or $(\mathbb{Z}_2)^3$. We omit the details. □

(A4.2) **Lemma.** *Here are the generating sets the need to be considered in each of these groups, in order to show that all of their connected Cayley graphs have hamiltonian cycles:*

(1a) $S = \{x, y\}$

(1b) $S = \{xw, y\}$ *or* $S = \{xw, yw^2\}$

(1c) $S = \{xz, yz'\}$ *or* $S = \{xz, xz', y\}$ *or* $S = \{x, yz, yz'\}$ *or* $S = \{x, yz, y'z'\}$

(1d) $S = \{x, y, z\}$ *or* $S = \{x, y, xz\}$

(1e) *none*

(1f) $S = \{x, iw\}$ *or* $S = \{xw, iw\}$ *or* $S = \{xw^2, iw\}$ *(note that* $|iw| = 2$*, because* $i^2 = w^2$*),*

(2a) *See Proposition A3.1.*

(2b) $S = \{a, y\}$ *or* $S = \{a, ay\}$ *or* $S = \{a, a^2y\}$,
*where* $a$ *acts on* $A_4$ *via the* 4*-cycle* $(1\,2\,3\,4)$*, and* $y$ *is the* 3*-cycle* $(1\,2\,3)$*,*

(2c) $S = \{f, ti\}$ *or* $S = \{f, fti\}$ *or* $S = \{fi, t\}$ *or* $S = \{fi, fti\}$.

(2d) $S = \{x, yi\}$ *or* $S = \{x, xyi\}$ *or* $S = \{xi, y\}$ *or* $S = \{xi, xyi\}$.

**Proof.** We use $Q$ to denote a Sylow 2-subgroup of $G$.

(1a) We may assume $S$ contains an element of $Q$, for otherwise we may assume $S \subset xQ$, so Theorem 2.10 applies. Thus, we may assume $y \in S$. Also, since some element of $S$ must generate $G/Q$, we may assume $x \in S$. So $S = \{x, y\}$.

(1b) We may assume $S$ contains an element of $Q$, for otherwise we may assume $S \subset xQ$, so Theorem 2.10 applies. Furthermore, since $(yw)^2$ is an element of order 2 in the center of $G$, we may assume $yw \notin S$. So either $y \in S$ or $yw^2 \in S$.

Now, let $s \in S \setminus A_4$. Replacing $\mathbb{Z}_3$ by a conjugate, we may assume $s = x^i w$. Since we may assume $s \notin Z(G)$ (otherwise Lemma 2.6(1) applies), we may assume $i = 1$. So $S = \{xw, y\}$ or $\{xw, yw^2\}$.

(1c) Since $S$ must generate $G/A_4$, we may assume there exist $a, b \in S$ with $a \in A_4 z$ and $b \in A_4 z'$.

If $a, b \in Q$, then we may assume $x \in S$, so $S = \{x, yz, yz'\}$ or $\{x, yz, y'z'\}$.

We may now assume $a = xz$. If $y \in Q$, then $S = \{xz, yz'\}$. Otherwise, we may assume $b = xz'$ or $xyz'$. In the latter case, we have $S = \{xz, yz'\}$. In the former case, let $c$ be the third element of $S$. We may assume $c \in Q$, for otherwise $S \subset xQ$, so Theorem 2.10 applies. Then we may assume $c \in Q \cap A_4$, for otherwise a previous case applies. So we may assume $c = y$, so $S = \{xz, xz', y\}$.

(1d) We may assume $x \in S$, since $S$ contains a generator of $G/Q$. And we may assume $S$ contains an element of $Q$ (otherwise we could assume $S \subset xQ$, so Theorem 2.10 applies). Thus, we may assume $y \in S$. Now, we may assume the third element of $S$ is in either $Q$ or $xQ$. So $S = \{x, y, z\}$ or $\{x, y, xz\}$.

(1e) We may assume $S \cap \mathbb{Z}_2 = \emptyset$, for otherwise Lemma 2.6(1) applies. Then we may assume $S \cap (Q_8 \times \mathbb{Z}_2) = \emptyset$, for otherwise Lemma 2.6(1) applies with $N = \mathbb{Z}_2$. Then (by replacing some generators by their inverses), we may assume $S \subset x(Q_8 \times \mathbb{Z}_2)$. So Theorem 2.10 applies.

(1f) We may assume there exists $a \in S \cap (Q_8 \times \mathbb{Z}_2) = \emptyset$, for otherwise (by replacing some generators by their inverses), we could assume $S \subset x(Q_8 \times \mathbb{Z}_2)$, and then Theorem 2.10 would apply. We may assume $|a| = 2$, for otherwise Corollary 2.3 applies (with $N = \langle w^2 \rangle$). So we may assume $a = iw$.

Now let $b \in S$ be a generator of $G/(Q_8 \times \mathbb{Z}_4)$. Replacing $x$ by a conjugate, we may assume $b = xi^{2k}w^{\ell} = xw^{\ell'}$. By passing to the inverse, we may assume $0 \le \ell' \le 2$. Note that $\langle a, b \rangle = G$, so $S = \{a, b\}$.

(2a) See Proposition A3.1.

(2b) Let $a \in S \smallsetminus A_4$. Then $|a| = 4$, so $G = \langle a \rangle \ltimes A_4$. We may assume $a^2$ is not in the center of $G$, for otherwise Corollary 2.3 applies. So $a$ acts on $A_4$ via conjugation by a 4-cycle, which we may assume is $(1\,2\,3\,4)$.

Choose $b \in S \smallsetminus Q$, where $Q$ is the Sylow 2-subgroup containing $a$. Then $b = a^i y$, where $y \in A_4$. Passing to the inverse, we may assume $0 \le i \le 2$. Furthermore, since $y \notin Q$, we know $y$ is a 3-cycle. By cyclically renumbering, we may assume $y = (1\,2\,3)^{\pm 1}$.

- If $i = 0$, then we may assume $y = (1\,2\,3)$ (by possibly replacing $b$ with its inverse).
- If $i = 1$, then we may assume $y = (1\,2\,3)$, for otherwise $b^2 \in Z(G)$, so Corollary 2.3 applies.
- If $i = 2$, then we may assume $y = (1\,2\,3)$ (by possibly replacing $b$ with its inverse).

(2c) We may assume $S \cap Q_8 = \emptyset$, for otherwise Corollary 2.3 applies with $N = \langle i^2 \rangle$.

Let $\overline{S}$ be the image of $S$ in $G/\langle i^2 \rangle \cong S_4$, and note that $\overline{S}$ is a minimal generating set, because $\langle i^2 \rangle = \Phi(Q_8) \subset \Phi(G)$.

Let $a \in \overline{S}$. There is some odd permutation in $\overline{S}$, so we may assume $a$ is either $(1\,2) = \overline{f}$ or $(1\,2\,3\,4) = \overline{fi}$. Let $b \in \overline{S} \smallsetminus \langle a, \overline{Q_8} \rangle$.

**Case 1.** *Assume* $a = (1\,2)$. If $\langle a, b \rangle \ncong D_6$, then $\langle a, b \rangle = G$; we may assume $b = \overline{f^k ti}$ (where $k \in \{0, 1\}$).

We may now assume $\langle a, b \rangle \cong D_3$, so $b = f^k t i^{2\ell}$. Then there must be a third element $c$ of $\overline{S}$, of the form $f^{k'} t^{\ell'} i$. We must have $\ell' = 0$, for otherwise $\langle a, c \rangle = \langle f, ti \rangle = G$. Then, since $c \notin Q_8$, we must have $k = 1$, so $c = \overline{fi}$. Then $\langle b, c \rangle = G$, contradicting the minimality of $S$.

**Case 2.** *Assume* $a = (1\,2\,3\,4) = \overline{fi}$. Then $\langle a, b \rangle = G$. And $b$ is either a 3-cycle, which we may take to be $(1\,2\,3) = \overline{t}$, or a 4-cycle, which we may take to be $(1\,3\,2\,4) = \overline{fti}$ (after conjugating by a power of $a$ and perhaps passing to the inverse).

(2d) Since $G/\langle i^2\rangle = G/\Phi(G) \cong S_4$, the arguments of (2c) apply. □

## A5. Proof of Proposition 3.4

**Proof.** We consider the generating sets listed in Lemma A4.2.

(1a) A hamiltonian cycle in the quotient multigraph $P\backslash\mathrm{Cay}(G;S)$ is:

$$\big(y^2, x, y^3, x^{-1}, y^{-3}, x, y^{-3}, x^{-1}, y\big).$$

It passes through the vertices in the order:

$$P, Py, Py^2, Pz^2, Pyz^2, Py^2z^2, Py^3z^2, Py^3z, Py^2z, Pyz, Pz, Py^3z^3, Py^2z^3, Pyz^3, Pz^3, Py^3, P.$$

The edge between $Py^2z^3$ and $Pyz^3$ is a double edge, coming from both $y^{-1}$ and $x$, so Lemma 2.4 provides a hamiltonian cycle in $\mathrm{Cay}(G;S)$.

(1b) For each of the two generating sets, we find a hamiltonian cycle in the quotient multigraph $P\backslash\mathrm{Cay}(G;S)$ whose endpoint in $G$ is $x^{-1}$. This generates $P$, so Lemma A2.2 provides a hamiltonian cycle in $\mathrm{Cay}(G;S)$.

For the generating set $\{xw, y\}$, the desired hamiltonian cycle in the quotient multigraph is:

$$\big(y, (xw)^3, (y, (xw)^{-1})^2, ((xw)^{-1}, y)^2, (xw)^{-2}, y, (xw)^{-1}\big).$$

This passes through the vertices in the order:

$$P, Py, Pwy', Pw^2yy', Pw^3y, Pw^3, Pw^2, Pw^2y,$$
$$Pwyy', Py', Pyy', Pw^3y', Pw^3yy', Pw^2y', Pwy, Pw, P.$$

The endpoint in $G$ is $yx^3yx^{-1}yx^{-2}yx^{-1}yx^{-2}yx^{-1} = x^{-1}$, as claimed.

For the generating set $\{xw, yw^2\}$, the desired hamiltonian cycle in the quotient multigraph is:

$$\big(yw^2, (xw)^{-1}, yw^2, xw, (yw^2, (xw)^{-1})^3, yw^2, xw, (yw^2, (xw)^{-1})^2\big).$$

This passes through the vertices in the order:

$$P, Pw^2y, Pwyy', Pw^3y', Pyy', Pw^2y', Pwy, Pw^3,$$
$$Pw^2, Py, Pw^3yy', Pwy', Pw^2yy', Py', Pw^3y, Pw, P.$$

The endpoint in $G$ is $yx^{-1}yxyx^{-1}yx^{-1}yx^{-1}yxyx^{-1}yx^{-1} = x^{-1}$, as claimed.

(1c) For each of the first two generating sets, we find a hamiltonian cycle in the quotient multigraph $P\backslash\mathrm{Cay}(G;S)$ that uses a double edge, so Lemma 2.4 provides a hamiltonian cycle in $\mathrm{Cay}(G;S)$.

- If $S = \{xz, yz'\}$, the desired hamiltonian cycle in $P\backslash\mathrm{Cay}(G;S)$ is:

  $$\big((yz', (xz)^{-2})^2, yz', xz, (yz', (xz)^2)^2, yz', xz$$

  This passes through the vertices in the order:

  $$P, Pyz', Pyy'zz', Py'z', Pyy', Py'z, Py, Pz', Pzz',$$
  $$Pyz, Py', Pyy'z, Py'zz', Pyy'z', Pyzz', Pz, P.$$

  The edge between $Pz$ and $P$ is a double edge, coming from both $xz$ and $(xz)^{-1}$.

- If $S = \{xz, xz', y\}$, the desired hamiltonian cycle in $P\backslash\mathrm{Cay}(G;S)$ is:

$$\big(y, (xz)^2, (xz')^{-1}, (xz)^2, y, xz, y, (xz)^{-2}, xz', (xz)^{-2}, y, xz\big).$$

  This passes through the vertices in the order:

$$P, Py, Py'z, Pyy', Py'z', Pyy'zz', Pyz', Pz', Pzz',$$
$$Pyzz', Pyy'z', Py'zz', Pyy'z, Py', Pyz, Pz, P.$$

  The edge between $Pz$ and $P$ is a double edge, coming from both $xz$ and $(xz)^{-1}$.

For the other two generating sets, we find a hamiltonian cycle in $\mathrm{Cay}\big(G/\langle z'\rangle; S\big)$ whose endpoint is $z'$, so the Factor Group Lemma (2.1) provides a hamiltonian cycle in $\mathrm{Cay}(G;S)$.

- If $S = \{x, yz, yz'\}$, the desired hamiltonian cycle in $\mathrm{Cay}\big(G/\langle z'\rangle; S\big)$ is:

$$\big((x^{-1}, yz')^2, yz, yz', x^{-1}, yz', yz, x^{-1}, yz', yz, yz', x^{-1}, yz', (x, yz')^2, yz, yz', x, yz', x^{-1}\big).$$

  This passes through the vertices of the quotient graph in the order:

$$e, x^{-1}, x^{-1}y, xyy', xy', xyy'z, xy'z, yz, z, y, x^{-1}yy', x^{-1}y', x^{-1}yy'z,$$
$$x^{-1}y'z, xyz, xz, x^{-1}z, x^{-1}yz, y'z, yy'z, y', yy', xy, x, e.$$

  Since $z'$ is in the center of $G$ and there are 11 edges that use $yz'$ in this cycle, the endpoint in $G$ is $z'$, as claimed.

- If $S = \{x, yz, y'z'\}$, the desired hamiltonian cycle in $\mathrm{Cay}\big(G/\langle z'\rangle; S\big)$ is:

$$\big(x^2, yz, x^{-2}, yz, (x^2, yz)^2, x, yz, x^{-2}, yz, x^2, yz, x^{-2}, yz, y'z'\big).$$

  This passes through the vertices of the quotient graph in the order:

$$e, x, x^{-1}, x^{-1}yz, xyy'z, y'z, yy', xy, x^{-1}y', x^{-1}yy'z, yz, xy'z, xyy',$$
$$x^{-1}y, x^{-1}z, xz, z, y, xy', x^{-1}yy', x^{-1}y'z, xyz, yy'z, y', e.$$

  Since $z'$ is in the center of $G$ and there is just one edge that uses $y'z'$ in this cycle, the endpoint in $G$ is $z'$, as claimed.

(1d) For each of the generating sets, we find a hamiltonian cycle in the quotient multigraph $P\backslash\mathrm{Cay}(G;S)$ that uses a double edge, so Lemma 2.4 provides a hamiltonian cycle in $\mathrm{Cay}(G;S)$.

- If $S = \{x, y, z\}$, the desired hamiltonian cycle in $P\backslash\mathrm{Cay}(G;S)$ is:

$$\big(y, x, y, z, y, x^{-1}, y, z\big)^2$$

  This passes through the vertices in the order:

$$P, Py, Py', Pyy', Pyy'z, Py'z, Pyzz', Pzz', Pz',$$
$$Pyz', Py'zz', Pyy'zz', Pyy'z', Py'z', Pyz, Pz, P.$$

  The edge between $Py'$ and $Pyy'$ is a double edge, coming from both $y$ and $x$.

- For the generating set $\{x, y, xz\}$, the desired hamiltonian cycle in the coset graph is:

$$\big(y, x^{-2}, (xz)^{-1}, x^2, y, x^2, xz, x^2, y, x^2, (xz)^{-1}\big)$$

  This passes through the vertices in the order:

$$P, Py, Pyy', Py', Pyzz', Py'z, Pyy'z', Py'z', Pyy'zz',$$
$$Pyz, Py'zz', Pyy'z, Pyz', Pz', Pzz', Pz, P.$$

The edge between $Pzz'$ and $Pz$ is a double edge, coming from both $x$ and $(xz)^{-1}$.

(1e) Nothing needs to be done.

(1f) For the first generating set, $\{x, iw\}$, a hamiltonian cycle in $\mathrm{Cay}\big(G/\langle w^2\rangle; S\big)$ is:

$$\big((x^2, iw)^2, (x^{-2}, iw)^2\big)^2.$$

This passes through the vertices in the order:

$e, x, x^2, x^2iw, jw, xkw, xj, i, x^2k, x^2jw, xiw, kw, j, xk, x^2i, x^2w, w, xw, xi, k, x^2j, x^2kw, xjw, iw, e.$

The endpoint in $G$ is

$$\begin{aligned}\big((x^2iw)^2(x^{-2}iw)^2\big)^2 &= \big((x^2i)^2(x^{-2}i)^2\big)^2\\ &= (xjx^{-1}kw^2)^2\\ &= j^2 = w^2,\end{aligned}$$

so the Factor Group Lemma (2.1) provides a hamiltonian cycle in $\mathrm{Cay}(G; S)$.

For the generating set $\{xw, iw\}$, a hamiltonian cycle in the quotient multigraph $P\backslash\mathrm{Cay}(G; S)$ is:

$$\big((xw)^3, iw, (xw)^4, iw, (xw)^{-1}, iw, (xw)^4, iw\big).$$

This passes through the vertices in the order:

$P, Pw, Pw^2, Pw^3, Pi, Pjw, Pkw^2, Piw^3, Pj, Pkw^3, Pjw^2, Pkw, Piw^2, Pjw^3, Pk, Piw, P.$

The endpoint in $G$ is

$$\begin{aligned}\big(xw)^3iw(xw)^4iw(xw)^{-1}iw(xw)^4iw &= ixix^{-1}ixiw^2\\ &= ikixiw^2 = kxiw^2 = xi^2w^2 = x.\end{aligned}$$

This generates $P$, so Lemma A2.2 applies..

For the generating set $\{xw^2, iw\}$, a hamiltonian cycle in the quotient multigraph $P\backslash\mathrm{Cay}(G; S)$ is:

$$\big((xw^2, iw)^5, ((xw^2)^{-1}, iw)^2, xw^2, iw\big).$$

This passes through the vertices in the order:

$P, Pw^2, Piw^3, Pjw, Pk, Piw^2, Pw, Pw^3, Pi, Pjw^2, Pkw, Pjw^3, Pkw^2, Pj, Pkw^3, Piw, P$

The edge between $P$ and $Pw^2$ is a double edge, coming from both $xw^2$ and $(xw^2)^{-1}$), so Lemma 2.4 applies.

(2a) See Proposition A3.1.

(2b) Let $s = (12)(34)$ and $t = (14)(23)$. Note that $\langle s, t\rangle$ is a Sylow 2-subgroup of $A_4$, and that $s^y = t$ and $t^y = s^{y^2} = st$.

- For the generating set $S = \{a, y\}$,

$$\big((a^3, y, a^{-3}, y^{-1})^2, a^3, y, (a^3, y^{-1})^2, a^3, y, a^{-3}, y, a^{-3}, y^{-1}, (a^3, y)^2\big)$$

  is a hamiltonian cycle in $\mathrm{Cay}(G; S)$. To verify this, we observe that it visits the vertices of the graph in the order

  $e, a, a^2, a^3, sy^2a^3, sy^2a^2, sy^2a, sy^2, sy, sya, sya^2, sya^3, ta^3, ta^2, ta, t, ty^2, ty^2a, ty^2a^2, ty^2a^3,$
  $ya^3, y, ya, ya^2, sa^2, sa^3, s, sa, stya, stya^2, stya^3, sty, sty^2, sty^2a^3, sty^2a^2, sty^2a, tya, ty,$
  $tya^3, tya^2, sta^2, sta^3, st, sta, y^2a, y^2a^2, y^2a^3, y^2, e.$

- For the generating set $S = \{a, ay\}$, let $H = \langle stya^2 \rangle = \{e, stya^2, sy, sta^2, ty^2, stya^2\}$, and note that $H$ is a cyclic subgroup of order 6. A hamiltonian cycle in the quotient multigraph $H\backslash\mathrm{Cay}(G : S)$ is given by
$$\big(a^3, ay, a^{-3}, ay\big).$$
This visits the vertices in the order
$$H, Ha, Ha^2, Ha^3, Hy, Hya^3, Hya^2, Hya, H.$$
The endpoint in $G$ is
$$(a^3)(ay)(a^{-3})(ay) = ya^2y = y(y^{a^2})a^2 = y(sy)a^2 = (s^{y^2})y^2a^2 = sty^2a^2,$$
which generates $\langle sty^2a^2 \rangle = H$. So Lemma A2.2 gives a hamiltonian cycle in $\mathrm{Cay}(G; S)$.
- For the generating set $S = \{a, a^2y\}$, a hamiltonian cycle in $\mathrm{Cay}\big(G/Z(G); S\big)$ is given by
$$\big((a^2y)^2, a, (a^2y)^2, a^{-1}, \big((a^2y)^2, a\big)^2, (a^2y)^{-2}, a^{-1}, (a^2y)^2, a, (a^2y)^2, a^{-1}, (a^2y)^{-2}, a\big).$$
To simplify the calculation of the endpoint in $G$, we first calculate the endpoint in $G/A_4$ to obtain
$$\begin{aligned}(a^2y)^2a(a^2y)^2a^{-1}\big((a^2y)^2a\big)^2(a^2y)^{-2}a^{-1}(a^2y)^2a(a^2y)^2a^{-1}(a^2y)^{-2}a &\equiv aa^{-1}a^2a^{-1}aa^{-1}a \\ &= a^2 \not\equiv e \pmod{A_4}.\end{aligned}$$
Since the endpoint is nontrivial in $G/A_4$, it is nontrivial in $G$, and thus, it is a nontrivial element of $Z(G) \cong \mathbb{Z}_2$. Therefore, it generates $Z(G)$, so the Factor Group Lemma (2.1) provides a hamiltonian cycle in $\mathrm{Cay}(G; S)$.

(2c)
- For the generating set $S = \{ti, f\}$, let $H = \langle k \rangle$. A hamiltonian cycle in the quotient multigraph $H\backslash\mathrm{Cay}(G; S)$ is given by
$$\Big(\big((ti)^2, f\big)^2, \big((ti)^{-2}, f\big)^2\Big).$$
It visits the vertices in the order
$$H, Ht, Hit^2, Hit^2f, Htf, Hif, Hi, Ht^2, Hit, Hitf, Ht^2f, Hf, H.$$
The endpoint in $G$ is
$$\big((ti)^2f\big)^2\big((ti)^{-2}f\big)^2 = (-it^2f)^2(ktf)^2 = ji = -k,$$
which generates $\langle k \rangle = H$. By Lemma A2.2, there is a hamiltonian cycle in $\mathrm{Cay}(G; S)$.
- For the generating set $S = \{f, fti\}$, let $H = \langle -t \rangle$, so $H$ is of order 6. A hamiltonian cycle in the quotient multigraph $H\backslash\mathrm{Cay}(G; S)$ is given by
$$\big((fti)^3, f, (fti)^{-3}, f\big).$$
It visits the vertices in the order
$$H, Hjf, Hj, Hkf, Hk, Hif, Hi, Hf, H.$$
The endpoint in $G$ is
$$(fti)^3f(fti)^{-3}f = (it^2f)f(kt^2f)f = it^2kt^2 = i(it^2)t^2 = -t,$$
which generates $\langle -t \rangle = H$. By Lemma A2.2, there is a hamiltonian cycle in $\mathrm{Cay}(G; S)$.

- For the generating set $S = \{fi, t\}$, let $H = \langle kt \rangle$, so $H$ is cyclic of order 6. A hamiltonian cycle in the quotient multigraph $H \backslash \mathrm{Cay}(G : S)$ is
$$\big((fi)^3, t, (fi)^{-3}, t^{-1}\big).$$
It visits the vertices in the order
$$H, Hjf, Hk, Hif, Hf, Hj, Hkf, Hi, H.$$
Its endpoint in $G$ is
$$(fi)^3 t (fi)^{-3} t^{-1} = (if) t (jf) t^{-1} = (if)(it)(ft^{-1}) = i(-jf)(tft^{-1}) = -kt,$$
which generates $\langle -kt \rangle = H$. By Lemma A2.2, there is a hamiltonian cycle in $\mathrm{Cay}(G; S)$.
- For the generating set $S = \{fi, fti\}$, let $H = \langle jt^2 \rangle$, so $H$ is cyclic of order 6. A hamiltonian cycle in the quotient multigraph $H \backslash \mathrm{Cay}(G : S)$ is
$$\big((fi)^3, fti, (fi)^{-3}, (fti)^{-1}\big).$$
It visits the vertices in the order
$$H, Hjf, Hk, Hif, Hi, Hf, Hj, Hkf, H.$$
Its endpoint in $G$ is
$$(fi)^3 (fti)(fi)^{-3}(fti)^{-1} = (if)(-kt^2 f)(jf)(-it^2 f) = (-jt)(-t) = jt^2,$$
which generates $\langle jt^2 \rangle = H$. By Lemma A2.2, there is a hamiltonian cycle in $\mathrm{Cay}(G; S)$.

(2d) For each of the four generating sets, we find a hamiltonian cycle in $\mathrm{Cay}\big(G/\langle x^2 \rangle; S\big)$ whose endpoint in $G$ is $x^2$. Then the Factor Group Lemma (2.1) provides a hamiltonian cycle in $\mathrm{Cay}(G; S)$. The first two generating sets contain the element $x$, which has order 2 in the quotient group but order 4 in $G$, so we do not need to calculate the endpoint in $G$, because Corollary 2.3 applies.

- For the generating set $\{x, yi\}$, the desired hamiltonian cycle in $\mathrm{Cay}\big(G/\langle x^2 \rangle; S\big)$ is:
$$\big((x, (yi)^2)^2, (x, (yi)^{-2})^2\big)^2.$$
This passes through the vertices of the quotient graph in the order:
$$e, x, xyi, xy^2k, yk, y^2, i, xj, xy^2j, xyj, y^2i, y, k, xk, xy, xy^2i, yj, y^2j, j, xi, xy^2, xyk, y^2k, yi, e.$$
- For the generating set $\{x, xyi\}$, the desired hamiltonian cycle in $\mathrm{Cay}\big(G/\langle x^2 \rangle; S\big)$ is:
$$\big(x, (xyi)^3, x, (xyi)^{-3}\big)^3.$$
This passes through the vertices of the quotient graph in the order:
$$e, x, yi, xj, yk, xy^2k, y^2j, xy^2i, y^2, xy, i, xyj, k, xk, yj, xi, y, xy^2, y^2i, xy^2j, y^2k, xyk, j, xyi, e.$$
- For the generating set $\{xi, y\}$, the desired hamiltonian cycle in $\mathrm{Cay}\big(G/\langle x^2 \rangle; S\big)$ is:
$$\big(y^2, xi, y^2, (xi)^{-1}, y^{-2}, xi, y^{-2}, (xi)^{-1}\big)^2.$$
This passes through the vertices of the quotient graph in the order:
$$e, y, y^2, xyi, xy^2j, xk, i, y^2k, yj, xy^2, xy, x, j, yk, y^2i, xyk, xy^2i, xj, k, y^2j, yi, xy^2k, xyj, xi, e.$$

The endpoint in $G$ is

$$\begin{aligned}\big(y^2xiy^2ix^3yxiyix^3\big)^2 &= (xyiy^2xjxy^2yjix^3)^2\\ &= (xyy^2kxx^3ikx)^2 = (xix)^2 = j^2 = x^2\end{aligned}$$

as claimed.

- For the generating set $\{xi, xyi\}$, the desired hamiltonian cycle in $\mathrm{Cay}\big(G/\langle x^2\rangle; S\big)$ is:

$$\big((xi)^{-1}, (xyi)^3, xi, (xyi)^{-3}\big)^3.$$

This passes through the vertices of the quotient graph in the order:

$$e, xj, yk, x, yi, xy^2k, y^2j, xy^2i, y^2, xyj, k, xy, i, xk, yj, xi, y, xy^2j, y^2k, xy^2, y^2i, xyk, j, xyi, e.$$

To calculate the endpoint of this cycle in $G$, notice that $(xyi)^2 = j$ has order 4, so the order of $xyi$ is 8, and $(xyi)^4 = x^2$. Now the endpoint of this cycle in $G$ is

$$\begin{aligned}\big(ix(xyi)^3xi(xyi)^{-3}\big)^3 &= (x^3jjxyixix^3yi)^3\\ &= (x^2yix^2jyi)^3 = (ykyi)^3 = (y^2i^2)^3 = x^2\end{aligned}$$

as claimed. □

## Additional references


[14] S. J. Curran, D. W. Morris, and J. Morris: Cayley graphs of order $16p$ are hamiltonian (preprint). http://arxiv.org/abs/1104.0081

[15] *GAP – Groups, Algorithms, and Programming.* http://www.gap-system.org

[16] D. Jungreis and E. Friedman: Cayley graphs on groups of low order are hamiltonian (unpublished).

[17] R. A. Rankin: A campanological problem in group theory II, *Proc. Camb. Phil. Soc.* 62 (1966) 11–18.



Department of Mathematics, University of Pittsburgh at Johnstown, Johnstown, PA 15904, USA

*E-mail address*: SJCurran@pitt.edu

Department of Mathematics and Computer Science, University of Lethbridge, Lethbridge, Alberta, T1K 3M4, Canada

*E-mail address*: Dave.Morris@uleth.ca, http://people.uleth.ca/~dave.morris/

Department of Mathematics and Computer Science, University of Lethbridge, Lethbridge, Alberta, T1K 3M4, Canada

*E-mail address*: Joy.Morris@uleth.ca, http://people.uleth.ca/~morris/
